# Supplementary material for: Distributed Multigrid Neural Solvers on Megavoxel Domains
Source: arXiv:2104.14538 source file (2021-04-29)
Supplement: Supplementary file 1 [file appendix.tex]

\section{Appendix}

\subsection{Batch size effect on convergence}
\textcolor{blue}{We continue exploring the effect of batch-size on convergence rates of both first order optimizers (SGD) as well as second order optimizers (L-BFGS) both of which are implemented in a data parallel way in SciDDL. Fig.~\ref{fig:loss-epoch-plots-128x128} plots the loss evolution with training epochs for a $128 \times 128$ DiffNet model that was trained on 1 node on Nova. These results are consistent with those shown in Fig.~\ref{fig:loss-epoch-plots-64x64} for a $64 \times 64$ resolution DiffNet model, where L-BFGS optimizer is relatively insensitive to the batch-size ranges chosen. As expected, the second order method converges in fewer epochs, with similar reduction in loss happening within 30 training epochs as compared to 150 epochs for SGD. L-BFGS optimizers require larger memory (to evaluate the Hessian) which a distributed approach (like SciDDL or LBANN) can gracefully accommodate.}
\textcolor{blue}{The increased computational overhead results in increased time per epoch, and this is plotted in  Fig.~\ref{fig:loss-time-plots-128x128}.}

\begin{figure}[!ht]
    \centering
    \begin{minipage}{.4\textwidth}
  \begin{center}
  \begin{tikzpicture}
      \begin{axis}[
    %   xmode=log,
    %   ymode=log,
    %   log ticks with fixed point,
          width=0.99\linewidth, % Scale the plot to \linewidth
          height=4cm,
          xlabel={Epoch}, % Set the labels
          ylabel=$\log_{10}(L)$, % Set the labels
          legend style={at={(0.95,0.95)},anchor=north east,legend columns=2}, % Put the legend below the plot
          xmin=0,
          xmax=310,
          ymin=-1.5,
          ymax=1.0,
          grid=both,
          x tick label style={rotate=0,anchor=north}
        ]
        \addplot+ [mark=none,line width=1pt]
        table[x expr={(\thisrowno{1})},y expr={log10(\thisrowno{3})},col sep=space]{Data/batch_size_experiment/n-0128/sgd/log_processed_bs_8.txt};
        \addplot+ [mark=none,line width=1pt]
        table[x expr={(\thisrowno{1})},y expr={log10(\thisrowno{3})},col sep=space]{Data/batch_size_experiment/n-0128/sgd/log_processed_bs_16.txt};
        \addplot+ [mark=none,line width=1pt]
        table[x expr={(\thisrowno{1})},y expr={log10(\thisrowno{3})},col sep=space]{Data/batch_size_experiment/n-0128/sgd/log_processed_bs_32.txt};
        \addplot+ [mark=none,line width=1pt]
        table[x expr={(\thisrowno{1})},y expr={log10(\thisrowno{3})},col sep=space]{Data/batch_size_experiment/n-0128/sgd/log_processed_bs_64.txt};
        % \addplot+
        % table[x expr={(\thisrow{nodes})},y expr={\thisrow{L2_Err}},col sep=space]{results_data/case_7_diff_gaussian_adref/k_1e-2_etol_1e-4/case7_error_data_adref.txt};
        \legend{\scriptsize{BS=8}, \scriptsize{BS=16}, \scriptsize{BS=32}, \scriptsize{BS=64}}
        % \node[] at (axis cs: 100,1.5) {SGD};
      \end{axis}
    \end{tikzpicture}
    \subcaption{SGD}
    \label{fig:128x128-sgd-loss-epoch}
    \end{center}
    \end{minipage}
    \vskip 8pt
\begin{minipage}{.4\textwidth}
  \begin{center}
  \begin{tikzpicture}
      \begin{axis}[
    %   xmode=log,
    %   ymode=log,
    %   log ticks with fixed point,
          width=0.99\linewidth, % Scale the plot to \linewidth
          height=4cm,
          xlabel={Epoch}, % Set the labels
          ylabel=$\log_{10}(L)$, % Set the labels
          legend style={at={(0.95,0.95)},anchor=north east,legend columns=2}, % Put the legend below the plot
          xmin=0,
          xmax=200,
          ymin=-1.5,
          ymax=1.0,
          grid=both,
          x tick label style={rotate=0,anchor=north}
        ]
        \addplot+ [mark=none,line width=1pt]
        table[x expr={(\thisrowno{1})},y expr={log10(\thisrowno{3})},col sep=space]{Data/batch_size_experiment/n-0128/lbfgs/log_processed_bs_8.txt};
        \addplot+ [mark=none,line width=1pt]
        table[x expr={(\thisrowno{1})},y expr={log10(\thisrowno{3})},col sep=space]{Data/batch_size_experiment/n-0128/lbfgs/log_processed_bs_16.txt};
        \addplot+ [mark=none,line width=1pt]
        table[x expr={(\thisrowno{1})},y expr={log10(\thisrowno{3})},col sep=space]{Data/batch_size_experiment/n-0128/lbfgs/log_processed_bs_32.txt};
        \addplot+ [mark=none,line width=1pt]
        table[x expr={(\thisrowno{1})},y expr={log10(\thisrowno{3})},col sep=space]{Data/batch_size_experiment/n-0128/lbfgs/log_processed_bs_64.txt};
        % \addplot+
        % table[x expr={(\thisrow{nodes})},y expr={\thisrow{L2_Err}},col sep=space]{results_data/case_7_diff_gaussian_adref/k_1e-2_etol_1e-4/case7_error_data_adref.txt};
        \legend{\scriptsize{BS=8}, \scriptsize{BS=16}, \scriptsize{BS=32}, \scriptsize{BS=64}}
        % \node[] at (axis cs: 50,0.6) {L-BFGS};
      \end{axis}
    \end{tikzpicture}
    \subcaption{L-BFGS}
    \label{fig:128x128-lbfgs-loss-epoch}
    \end{center}
    \end{minipage}
    \caption{\ipoint{Loss vs. epoch for $128\times 128$ domain DiffNet with varying batch-size (BS). Second order optimizers (L-BFGS) show faster convergence rate and provide minimal convergence drift with higher batch-size.}}
    \label{fig:loss-epoch-plots-128x128}
\end{figure}

\vfill\break
\begin{figure}[!ht]
    \centering
    \begin{minipage}{.4\textwidth}
  \begin{center}
  \begin{tikzpicture}
      \begin{axis}[
    %   xmode=log,
    %   ymode=log,
    %   log ticks with fixed point,
          width=0.99\linewidth, % Scale the plot to \linewidth
          height=4cm,
          xlabel={time (sec)}, % Set the labels
          ylabel=$\log_{10}(L)$, % Set the labels
          legend style={at={(0.95,0.95)},anchor=north east,legend columns=2}, % Put the legend below the plot
          xmin=0,
          xmax=5000,
          ymin=-1.5,
          ymax=1.0,
          grid=both,
          x tick label style={rotate=0,anchor=north}
        ]
        \addplot+ [mark=none,line width=1pt]
        table[x expr={(\thisrowno{0})},y expr={log10(\thisrowno{3})},col sep=space]{Data/batch_size_experiment/n-0128/sgd/log_processed_bs_8.txt};
        \addplot+ [mark=none,line width=1pt]
        table[x expr={(\thisrowno{0})},y expr={log10(\thisrowno{3})},col sep=space]{Data/batch_size_experiment/n-0128/sgd/log_processed_bs_16.txt};
        \addplot+ [mark=none,line width=1pt]
        table[x expr={(\thisrowno{0})},y expr={log10(\thisrowno{3})},col sep=space]{Data/batch_size_experiment/n-0128/sgd/log_processed_bs_32.txt};
        \addplot+ [mark=none,line width=1pt]
        table[x expr={(\thisrowno{0})},y expr={log10(\thisrowno{3})},col sep=space]{Data/batch_size_experiment/n-0128/sgd/log_processed_bs_64.txt};
        % \addplot+
        % table[x expr={(\thisrow{nodes})},y expr={\thisrow{L2_Err}},col sep=space]{results_data/case_7_diff_gaussian_adref/k_1e-2_etol_1e-4/case7_error_data_adref.txt};
        \legend{\scriptsize{BS=8}, \scriptsize{BS=16}, \scriptsize{BS=32}, \scriptsize{BS=64}}
        % \node[] at (axis cs: 1500,1.4) {SGD};
      \end{axis}
    \end{tikzpicture}
    \subcaption{SGD}
    \label{fig:128x128-sgd-loss-time}
    \end{center}
    \end{minipage}
    \vskip 8pt
    \begin{minipage}{.4\textwidth}
  \begin{center}
  \begin{tikzpicture}
      \begin{axis}[
    %   xmode=log,
    %   ymode=log,
    %   log ticks with fixed point,
          width=0.99\linewidth, % Scale the plot to \linewidth
          height=4cm,
          xlabel={time (sec)}, % Set the labels
          ylabel=$\log_{10}(L)$, % Set the labels
          legend style={at={(0.95,0.95)},anchor=north east,legend columns=2}, % Put the legend below the plot
          xmin=0,
          xmax=25000,
          ymin=-1.5,
          ymax=1.0,
          grid=both,
          x tick label style={rotate=0,anchor=north}
        ]
        \addplot+ [mark=none,line width=1pt]
        table[x expr={(\thisrowno{0})},y expr={log10(\thisrowno{3})},col sep=space]{Data/batch_size_experiment/n-0128/lbfgs/log_processed_bs_8.txt};
        \addplot+ [mark=none,line width=1pt]
        table[x expr={(\thisrowno{0})},y expr={log10(\thisrowno{3})},col sep=space]{Data/batch_size_experiment/n-0128/lbfgs/log_processed_bs_16.txt};
        \addplot+ [mark=none,line width=1pt]
        table[x expr={(\thisrowno{0})},y expr={log10(\thisrowno{3})},col sep=space]{Data/batch_size_experiment/n-0128/lbfgs/log_processed_bs_32.txt};
        \addplot+ [mark=none,line width=1pt]
        table[x expr={(\thisrowno{0})},y expr={log10(\thisrowno{3})},col sep=space]{Data/batch_size_experiment/n-0128/lbfgs/log_processed_bs_64.txt};
        % \addplot+
        % table[x expr={(\thisrow{nodes})},y expr={\thisrow{L2_Err}},col sep=space]{results_data/case_7_diff_gaussian_adref/k_1e-2_etol_1e-4/case7_error_data_adref.txt};
        \legend{\scriptsize{BS=8}, \scriptsize{BS=16}, \scriptsize{BS=32}, \scriptsize{BS=64}}
        % \node[] at (axis cs: 5500,0.6) {L-BFGS};
      \end{axis}
    \end{tikzpicture}
    \subcaption{L-BFGS}
    \label{fig:128x128-lbfgs-loss-time}
    \end{center}
    \end{minipage}
    \caption{\ipoint{Loss vs. time for $128\times 128$ domain DiffNet shown in Fig.~\ref{fig:loss-epoch-plots-128x128}}}
    \label{fig:loss-time-plots-128x128}
\end{figure}

\clearpage
\subsection{Additional quantitative comparison between DiffNet and conventional PDE solvers}
\textcolor{blue}{In this subsection, we provide additional results over those shown in the main text to quantitatively compare the DiffNet inferences with conventional PDE solver technology. Figure~\ref{fig:plot-solutions-vs-x-t-1-resolution-512} plots the solution at a particular time instance ($t = 0.2$) where there is formation of shocks. Notice that the DiffNet solution is very close to the fully resolved FDM solution for the large wave-number case ($c= 13$), with increasingly large deviations as the wave-number is decreased.}

\begin{figure}[!ht]
    \centering
    \begin{minipage}[t]{.33\textwidth}
      \centering
      \begin{tikzpicture}
      \begin{axis}[
          width=0.99\linewidth, % Scale the plot to \linewidth
          %grid=major, % Display a grid
          %grid style={line width=.1pt, draw=gray!50}, % Set the style
          xlabel=$x$, % Set the labels
          ylabel=$u$,
          legend cell align={left},
          legend style={at={(0.98,0.02)},anchor=south east,legend columns=3}, % Put the legend below the plot
          xmin=-0.1,
          xmax=1.1,
        grid=both,
          x tick label style={rotate=0,anchor=north} % Display labels sideways
        ]
        \addplot+ [color=black,mark=none,line width=1.2pt]
        table[x expr={\thisrow{"arc_length"}},y expr={\thisrow{"u_ml"}},col sep=comma]{Data/solution_plots/line_cuts/n_512_c_3.csv};
        \addplot+ [color=red,mark=none]
        table[x expr={\thisrow{"arc_length"}},y expr={\thisrow{"u_fem"}},col sep=comma]{Data/solution_plots/line_cuts/n_512_c_3.csv};
        \addplot+ [color=blue,dashed,mark=none,line width=1pt]
        table[x expr={\thisrow{"arc_length"}},y expr={\thisrow{"u_fdm"}},col sep=comma]{Data/solution_plots/line_cuts/n_512_c_3.csv};
        \legend{\tiny{SciDDL}, \tiny{FEM},\tiny{FDM}}
      \end{axis}
    \end{tikzpicture}
    \end{minipage}
    % \vspace{0.5mm}
    % \vskip 5pt
    % \hspace{0.1mm}
    \\
    \begin{minipage}[t]{.33\textwidth}
      \centering
      \begin{tikzpicture}
      \begin{axis}[
          width=0.99\linewidth, % Scale the plot to \linewidth
          %grid=major, % Display a grid
          %grid style={line width=.1pt, draw=gray!50}, % Set the style
          xlabel=$x$, % Set the labels
          ylabel=$u$,
          legend cell align={left},
          legend style={at={(0.98,0.02)},anchor=south east,legend columns=3}, % Put the legend below the plot
          xmin=-0.1,
          xmax=1.1,
        grid=both,
          x tick label style={rotate=0,anchor=north} % Display labels sideways
        ]
        \addplot+ [color=black,mark=none,line width=1.2pt]
        table[x expr={\thisrow{"arc_length"}},y expr={\thisrow{"u_ml"}},col sep=comma]{Data/solution_plots/line_cuts/n_512_c_5.csv};
        \addplot+ [color=red,mark=none]
        table[x expr={\thisrow{"arc_length"}},y expr={\thisrow{"u_fem"}},col sep=comma]{Data/solution_plots/line_cuts/n_512_c_5.csv};
        \addplot+ [color=blue,dashed,mark=none,line width=1pt]
        table[x expr={\thisrow{"arc_length"}},y expr={\thisrow{"u_fdm"}},col sep=comma]{Data/solution_plots/line_cuts/n_512_c_5.csv};
        \legend{\tiny{SciDDL}, \tiny{FEM},\tiny{FDM}}
      \end{axis}
    \end{tikzpicture}
    \end{minipage}
    \begin{minipage}[t]{.33\textwidth}
      \centering
      \begin{tikzpicture}
      \begin{axis}[
          width=0.99\linewidth, % Scale the plot to \linewidth
          %grid=major, % Display a grid
          %grid style={line width=.1pt, draw=gray!50}, % Set the style
          xlabel=$x$, % Set the labels
          ylabel=$u$,
          legend cell align={left},
          legend style={at={(0.98,0.02)},anchor=south east,legend columns=1}, % Put the legend below the plot
          xmin=-0.1,
          xmax=1.1,
        grid=both,
          x tick label style={rotate=0,anchor=north} % Display labels sideways
        ]
        \addplot+ [color=black,mark=none,line width=1.2pt]
        table[x expr={\thisrow{"arc_length"}},y expr={\thisrow{"u_ml"}},col sep=comma]{Data/solution_plots/line_cuts/n_512_c_13.csv};
        \addplot+ [color=red,mark=none]
        table[x expr={\thisrow{"arc_length"}},y expr={\thisrow{"u_fem"}},col sep=comma]{Data/solution_plots/line_cuts/n_512_c_13.csv};
        \addplot+ [color=blue,dashed,mark=none,line width=1pt]
        table[x expr={\thisrow{"arc_length"}},y expr={\thisrow{"u_fdm"}},col sep=comma]{Data/solution_plots/line_cuts/n_512_c_13.csv};
        \legend{\tiny{SciDDL}, \tiny{FEM},\tiny{FDM}}
      \end{axis}
    \end{tikzpicture}
    \end{minipage}
    \hspace{0.1mm}
    \caption{\ipoint{The solution profile $u$ vs. $x$ at $t = 0.2$, compared for different methods. Resolution = $512\times 512$ and $c$ values are $3$ (top), $5$ (middle) and $13$ (bottom)}}
    \label{fig:plot-solutions-vs-x-t-1-resolution-512}
\end{figure}
